# Supplementary material for: Oxidation dynamics of ultrathin GaSe probed through Raman spectroscopy
Source: arXiv:1612.06907 ancillary file (2017-06-12)
Supplement: Supplementary file 1 [file supporting_info.pdf]

# Oxidation dynamics of ultrathin GaSe probed through Raman spectroscopy

## Supplementary Material

Alaric Bergeron,[1] John Ibrahim,[1] Richard Leonelli,[2] and Sebastien Francoeur[1]

[1]*Department of Engineering Physics, Polytechnique Montréal, Montréal H3T 1J4, Canada*

[2]*Department of Physics, Université de Montréal, Montréal H3T 1J4, Canada*

## SI. THERMAL OXIDATION DYNAMICS OF GASE

The dominant thermal oxidation pathways involving GaSe and oxygen are well known [1],

$$\mathrm{GaSe} + \tfrac{3}{4}\mathrm{O_2} \rightarrow \tfrac{1}{2}\mathrm{Ga_2O_3} + \mathrm{Se}, \tag{S1a}$$

$$\mathrm{GaSe} + \tfrac{1}{4}\mathrm{O_2} \rightarrow \tfrac{1}{3}\mathrm{Ga_2Se_3} + \tfrac{1}{6}\mathrm{Ga_2O_3}, \tag{S1b}$$

$$\mathrm{Ga_2Se_3} + \tfrac{3}{2}\mathrm{O_2} \rightarrow \mathrm{Ga_2O_3} + 3\mathrm{Se}. \tag{S1c}$$

Experimental studies have found that reaction (S1a) is enabled around 150-250 °C and that it dominates the other two at low temperatures. The production of $Ga_2Se_3$ through reaction (S1b) has been observed at temperature above 450 °C [1–3]. Reaction (S1c) is enabled at temperatures around 600-700 °C [1–3] and eventually consumes all the $\alpha$-$Ga_2Se_3$ produced through reaction (S1b). The final oxidation products are $\beta$-$Ga_2O_3$ and Se. Due to its high vapor pressure, Se produced through (S1a) and (S1c) is easily be lost by sublimation and is rarely observed in thermally oxidized samples [2, 3]. The $Ga_2O_3$ formed at these high temperatures is either amorphous, suboxidized (GaO, $Ga_2O$), or of poor crystalline quality [2, 3].

## SII. ESTIMATION OF LASER-INDUCED SAMPLE HEATING

Fig. S1 shows the evolution of $A_1^4$ measured from a thin GaSe flake as a function of exposure power in vacuum. The maximum observed energy variation is $0.6\,\mathrm{cm^{-1}}$ between the lowest and highest excitation powers. If all this variation were attributed to thermal effects, the net resulting change in temperature $\Delta T$ calculated from the first-order temperature dependence of $-0.014\,\mathrm{cm^{-1}\,K^{-1}}$ reported in Ref. 4 would be 43 K. Since the increase in temperature is largely independent of sample thickness[5], these results clearly establish that thermally activated mechanisms are of secondary importance as discussed in the main text.

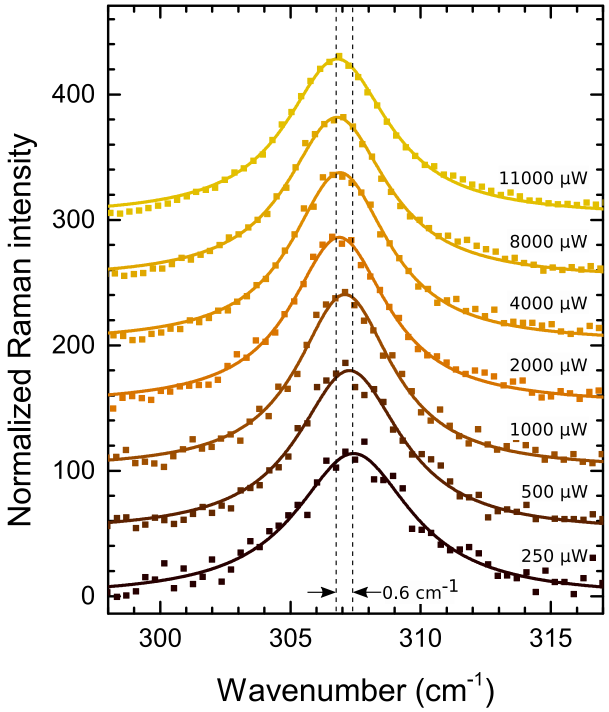


FIG. S1. Evolution of the energy position of GaSe ($A_1^4$) as a function of excitation power. Solid lines are Lorentzian fits used to extract the peak energy and points represent the measured data. The dashed lines shows the largest peak positions variation observed, which is between the lowest and highest .

## SIII. POLARIZED RAMAN MEASUREMENTS ON $Ga_2Se_3$ AND $Ga_2O_3$

The space group symmetry of the vacancy-ordered crystal $\alpha$-$Ga_2Se_3$ is $C_{2v}^{20}$. As a function of linear polarization angle $\theta$, the scattering efficiency of this $A_1$ mode is

$$I_{\parallel}(\theta) = (\alpha_i \cos^2\theta + \alpha_j \sin^2\theta)^2 \tag{S2}$$

$$I_{\perp}(\theta) = (\alpha_i - \alpha_j)^2, (\alpha_i \cos^2\theta \sin^2\theta), \tag{S3}$$

for co-polarized $k(\theta,\theta)\bar{k}$ and cross-polarized $k(\theta,\theta+\pi/2)\bar{k}$ configurations, respectively. In these equations, $\alpha_i$ and $\alpha_j$ are two of three diagonal Raman tensor elements selected by the measurement axis $k$. The polarization-resolved Raman intensity shown in Fig. S2(a) reveals a uniform response where no $\theta$ dependence can be identified in both configurations. This uniform response and the lack of extinction in cross-polarized configuration strongly suggests that the photo-induced $\alpha$-$Ga_2Se_3$ phase is polycrystalline.

Fig. S2(b) presents the polarization-resolved signal of the $A_g$ vibrational mode of $\beta$-

$Ga_2O_3$ observed at at 161 $cm^{-1}$. In a co-polarized configuration, the signal does not explicitly depend on the angle of polarization, just as the $\alpha$-$Ga_2Se_3$ ($A_1$) mode. In a cross-polarized configuration, the signal is too weak to be analyzed.

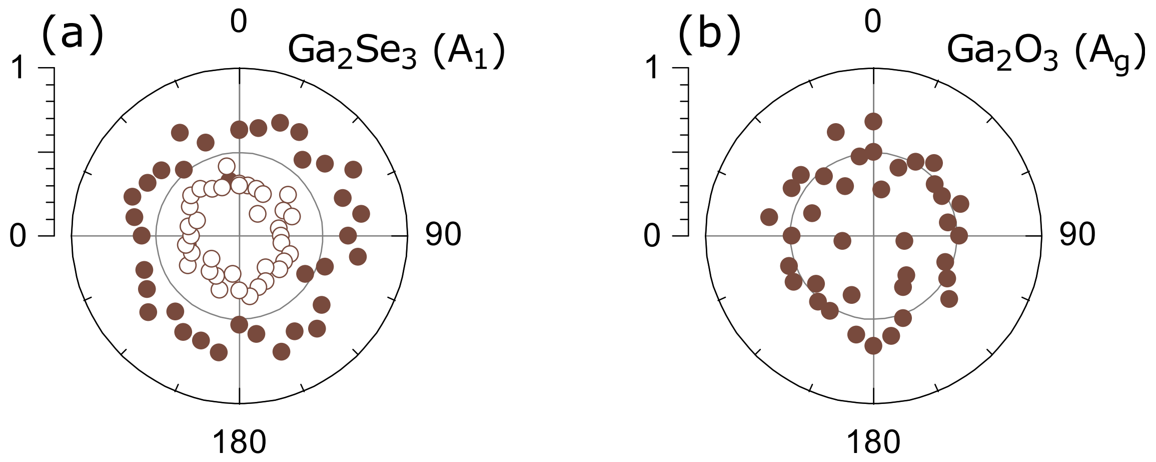


FIG. S2. Polarization-resolved Raman intensity from (a) $Ga_2Se_3$ $A_1$ and (b) $Ga_2O_3$ $A_g$ modes for co-polarized (full circles) and cross-polarized (empty circles) configurations.

## SIV. PHOTOLUMINESCENCE OF GaSe

As shown in Fig. S3, the well-defined and relatively narrow emission (6 nm FWHM) is replaced by a very broad emission uncharacteristic of a high-quality semiconductor. After 30 min, the luminescence signal has disappeared.

## SV. PHOTO-INDUCED OXIDATION UNDER OXYGEN AND WATER VAPOR

Controlled measurements were conducted using oxygen (99.999% purity, $<$ 3 ppm $H_2O$, $<$ 0.5 ppm total hydrocarbons content) and water vapor obtained from deionized water deoxygenated through several freeze-thaw cycles under vacuum. The oxygen and water vapor pressures in the sample chamber were controlled to be equivalent to their respective partial pressures in ambient atmosphere with 50% relative humidity. Results are shown in Fig. S4. As can be seen, oxygen and water vapor individually do not quench the Raman signal, but the simultaneous presence of both oxygen and water vapor invariably does irrespective of their introduction sequence. Simultaneously, the amorphous selenium vibrational mode

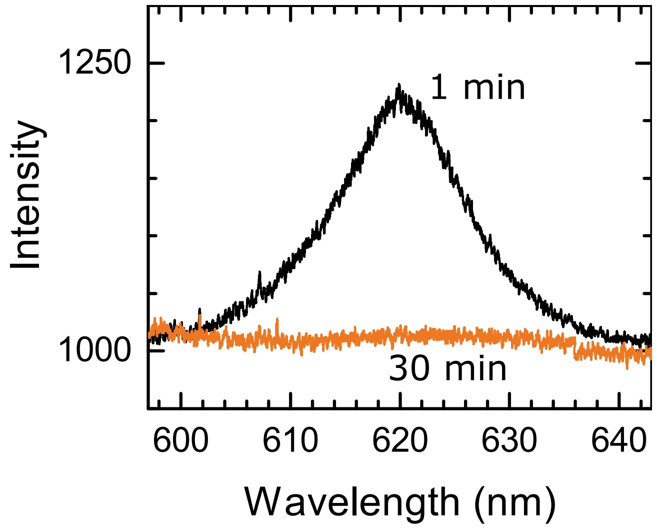


FIG. S3. Photoluminescence intensity of a 45 nm sample after 1 and 30 min of exposure in air.

appears at 257 $cm^{-1}$ and increases in intensity as those from GaSe disappear. This result clearly establishes the concurrent role of water and oxygen in the photo-induced oxidation process.

## SVI. CHARGE TRANSFER MODEL

The Marcus-Gerischer theory predicts that oxygen molecules solvated in water present an acceptor state positioned at $[E^0_{F,redox} + \lambda] = -3.1\,\mathrm{eV}$, where the renormalization energy of $\lambda = 1\,\mathrm{eV}$ is due to the fast reorganization of water molecules around oxygen[6, 7]. Fig. S5 illustrates the energy position of these acceptor states relatively to GaSe, which is characterized by an electron affinity of $-3.4\,\mathrm{eV}$ [8]. The significant overlap between the conduction band and acceptor states enables the charge transfer of photoexcited carriers in GaSe to the solvated $O_2$, yielding superoxide anions ($O_2^{\cdot-}$) [9]. The rate of this charge transfer is described by Eq. (2) of the main text.

[1] O. Balitskii and V. Savchyn, Materials Science in Semiconductor Processing **7**, 55 (2004).

[2] N. Berchenko, O. Balitskii, R. Lutsiv, V. Savchyn, and V. Vasyltsiv, Materials Chemistry and Physics **51**, 125 (1997).

[3] V. P. Savchyn and J. M. Stakhira, Physica Status Solidi (a) **156**, 113 (1996).

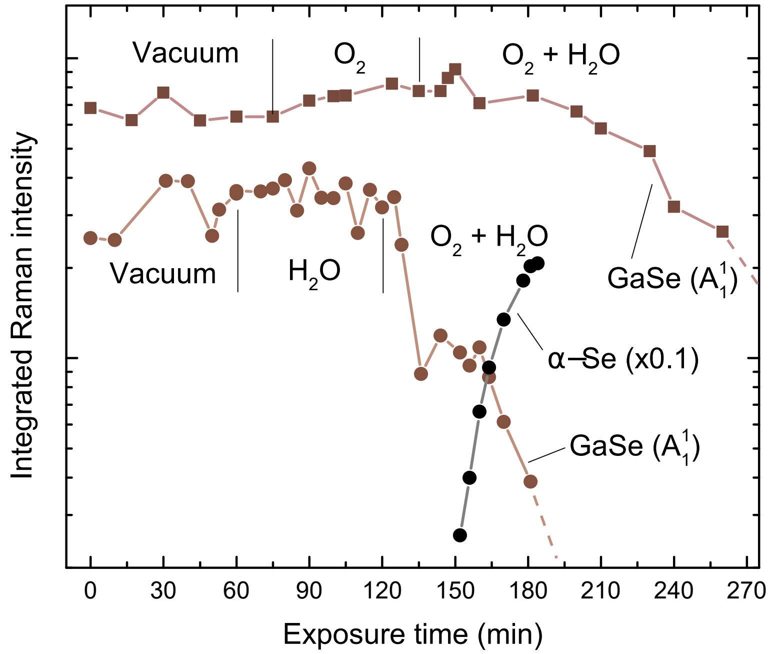


FIG. S4. Integrated Raman intensity of the GaSe $A_1^1$ vibrational mode as a function of exposure time under 1000 µW of 532 nm laser light in various environments: vacuum, $O_2$, oxygen-free $H_2O$ and $O_2 + H_2O$. The bottom curve also shows the associated appearance of the amorphous selenium Raman peak.


[4] N. Gasanly, A. Aydınlı, H. Özkan, and C. Kocabaş, Materials Research Bulletin **37**, 169 (2002).

[5] J. Judek, A. P. Gertych, M. Świniarski, A. Łapińska, A. Dużyńska, and M. Zdrojek, Scientific Reports **5**, 12422 (2015).

[6] P. L. Levesque, S. S. Sabri, C. M. Aguirre, J. Guillemette, M. Siaj, P. Desjardins, T. Szkopek, and R. Martel, Nano letters **11**, 132 (2011).

[7] A. Ignaczak, W. Schmickler, and S. Bartenschlager, Journal of Electroanalytical Chemistry **586**, 297 (2006).

[8] R. H. Williams and A. J. McEvoy, Physica Status Solidi (a) **12**, 277 (1972).

[9] A. Favron, E. Gaufres, F. Fossard, A.-L. Phaneuf-L'Heureux, N. Y.-W. Tang, P. L. Levesque, A. Loiseau, R. Leonelli, S. Francoeur, and R. Martel, Nat Mater **14**, 826 (2015).

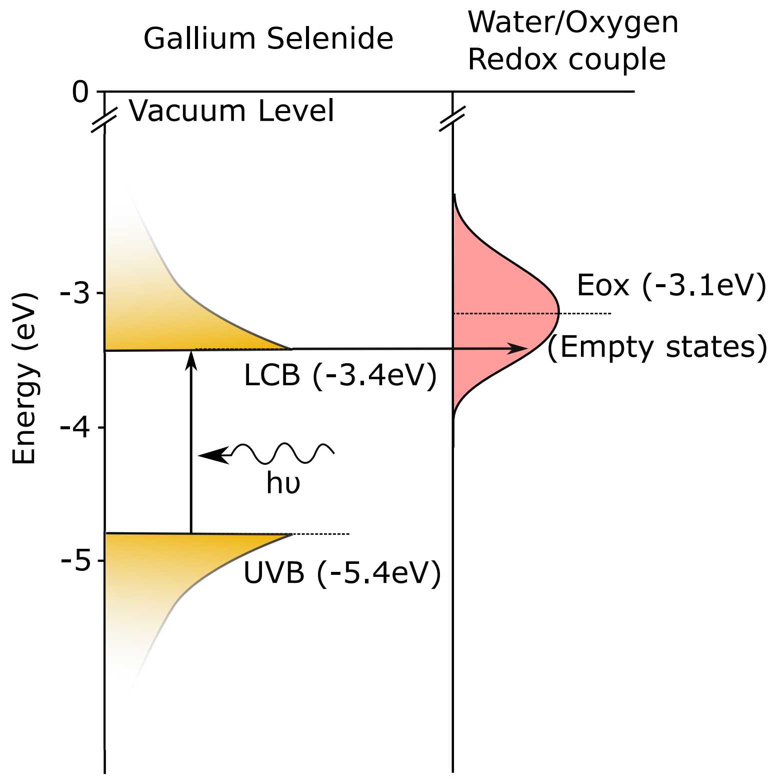


FIG. S5. Schematic of the charge transfer process from GaSe to aqueous oxygen. The band energies of GaSe and solvated oxygen molecules are illustrated relatively to vacuum [6, 8]. The vertical arrow represents the photoexcitation of a carrier from the upper valence band (UVB) to the lowest conduction band (LCB). Horizontal arrow indicates electron transfer from the LCB to the aqueous oxygen.
